# Supplementary material for: Prompt Cache: Modular Attention Reuse for Low-Latency Inference
Source: arXiv:2311.04934 source file (2024-04-25)
Supplement: Supplementary file 1 [file appendix.tex]

\newpage

\section{Appendix}
\subsection{Schema Files Used for Evaluation in Section 5.3}

\setcounter {page} {1}

In this appendix, we provide the pruned schema files that were employed during our evaluations as described in Section 5.3.

\subsubsection{Code Schema}

\begin{lstlisting}[style=xmlstyle]
<schema name="code-generation-game">
  <system>
    You are a sophisticated ...
  </system>
  <user> 
    Please read the given source files... 
    <module name="unit.py">
      class Unit:
      ...
    </module>
    <module name="player.py">
      class Player:
      ...
    </module>
    <module name="game.py">
      class Game:
      ...
    </module>
    <module name="database.py">
      class Database:...
    </module>
  </user>
  <assistant>
    I have read and ...
  </assistant>
</schema>
\end{lstlisting}

\subsubsection{Travel Schema}

\begin{lstlisting}[style=xmlstyle]
<schema name="travel">
  <system>
    You are a world-renowned travel planner ...
  </system>
  <user>
    <module name="travel-plan"> I'm gearing up for a memorable escape ... 
      <parameter name="duration" length="5" /> 
      ... 
      <union>
        <module name='domestic'> My eyes are set ... 
          <parameter name="city" length="10" />
           Given its domestic charm ...
        </module>
        <module name="overseas"> I'm yearning to tread ... 
          <union>
            <module name="maldives">
              The Maldives beckons ...
            </module>
            <module name="amazon">
              The vast expanse of the Amazon...
            </module>
            <module name="sahara">
              The golden embrace of the Sahara ...
            </module>
            <module name="tokyo">
              Tokyo, Japan's bustling capital,...
            </module>
            <module name="rome">
              The eternal city of Rome...
            </module>
            <module name="capetown">
              Cape Town, nestled at the foot...
            </module>
            <module name="sydney">
              Sydney, the shimmering jewel of Australia...
            </module>
            <module name="buenosaires">
              Buenos Aires, Argentina..
            </module>
          </union>
        </module>
      </union>
    </module>
  </user>
  <assistant>
    I'd love to help. I've carefully read the city ...
  </assistant>
</schema>
\end{lstlisting}

\subsubsection{Personalization Schema}

\begin{lstlisting}[style=xmlstyle]
<schema name="personalization-education">
  <system>Dialogues between people...
  </system>
  <user> **Tailor learning content ... 
    <union>
      <module name="elementary">
        The elementary phase ..
      </module>
      <module name="middle-school">
        As students transition...
      </module>
      <module name="high-school">
        High school acts...
      </module>
      <module name="college">
        College is a transformative ...
      </module>
      <module name="graduate-school">
        Graduate school signifies ...
      </module>
      <module name="adult-education">
        In an ever-evolving world,...
      </module>
    </union>
    2. Subject proficiency ...
    <union>
      <module name="beginner">
        A beginner is often at ...
      </module>
      <module name="intermediate">
        An intermediate learner...
      </module>
      <module name="advanced">
        An advanced learner...
      </module>
      <module name="expert">
        An expert stands at...
      </module>
    </union>
    3. Recent learning history
    <union>
      <module name="recently-studied">
        If a topic was engaged...
      </module>
      <module name="studied-a-month-before">
        Topics encountered a ...
      </module>
      <module name="studied-6-months-before">
        Half a year is ample ...
      </module>
      <module name="studied-a-year-before">
        As the year mark ...
      </module>
      <module name="studied-10-years-before">
        A decade is a substantial...
      </module>
      <module name="never-studied">
       Venturing into entirely ...
      </module>
    </union>
    4. Learning style...
     <union>
      <module name="visual">
        Visual learners ...
      </module>
      <module name="auditory">
        For auditory learners...
      </module>
      <module name="kinesthetic">
        Kinesthetic learners ...
      </module>
      <module name="reading">
        Those who identify ...
      </module>
      <module name="multimodal">
        Multimodal learners ...
      </module>
    </union>
    5. Preferred assessment type 
     <union>
      <module name="multiple-choice">
       Multiple choice assessments ...
      </module>
      <module name="essay">
        Essay assessments...
      </module>
      <module name="oral-presentation">
        This assessment type ...
      </module>
      <module name="group-projects">
        A testament to collaborative...
      </module>
      <module name="self-assessment">
        Taking a step back ...
      </module>
    </union>
    6. Motivation level Motivation...
    <union>
      <module name="high-intrinsic-motivation">
        Learners with a high intrinsic motivation ...
      </module>
      <module name="high-extrinsic-motivation">
        While some are driven by ...
      </module>
      <module name="needs-encouragement">
        Some learners, while capable,...
      </module>
      <module name="lacks-direction">
        This category encompasses...
      </module>
    </union>
    Ready to tailor the content? </user>
  <assistant>
    Content tailored ...
  </assistant>
</schema>
\end{lstlisting}

\subsection{Complete Benchmarks Results}
In this subsection, we provide complete results of the benchmark that we conducted in \S5---the following four datasets are added: \code{Qasper}, \code{MFQA}, \code{HotpotQA}, and \code{PCount} (total 12 datasets). We employ LongBench suite to measure time-to-first-token (TTFT) latency and accuracy. For the complete system environment setup, see \S5.1.

\paragraph{Latency benefits on GPU} \autoref{fig:appendix-gpu-latency-rtx4090} to \autoref{fig:appendix-gpu-latency-a40} show that the TTFT latency reduction across all dataset follows the same trend reported in \S5. The latency reduction ranges from $1.5\times$ to $3.1\times$ when \modus are stored in CPU memory, and from $3.7\times$ to $11.7\times$ when employing GPU memory.

\paragraph{Latency benefits on CPU} The latency reduction on CPU also follow the same trend as \S5.2, as shown in \autoref{fig:appendix-cpu-latency-intel} and \autoref{fig:appendix-cpu-latency-amd}. The latency improvement  ranges from $9.3\times$ to $63.7\times$ across CPU configurations and dataset. As discussed in \S5.4, the latency reduction decreases as the non-cacheable portion of prompt and response increases.

\paragraph{Quality of responses} We measure accuracy in dataset-specific metric as shown in \autoref{table:appendix_accuracy}. Across datasets and metrics, \tech maintains negligible performance degradation compared to the baseline, \kvcache.

\begin{figure*}[]
\centering
\vspace{-10pt}
\includegraphics[width=0.95\textwidth]{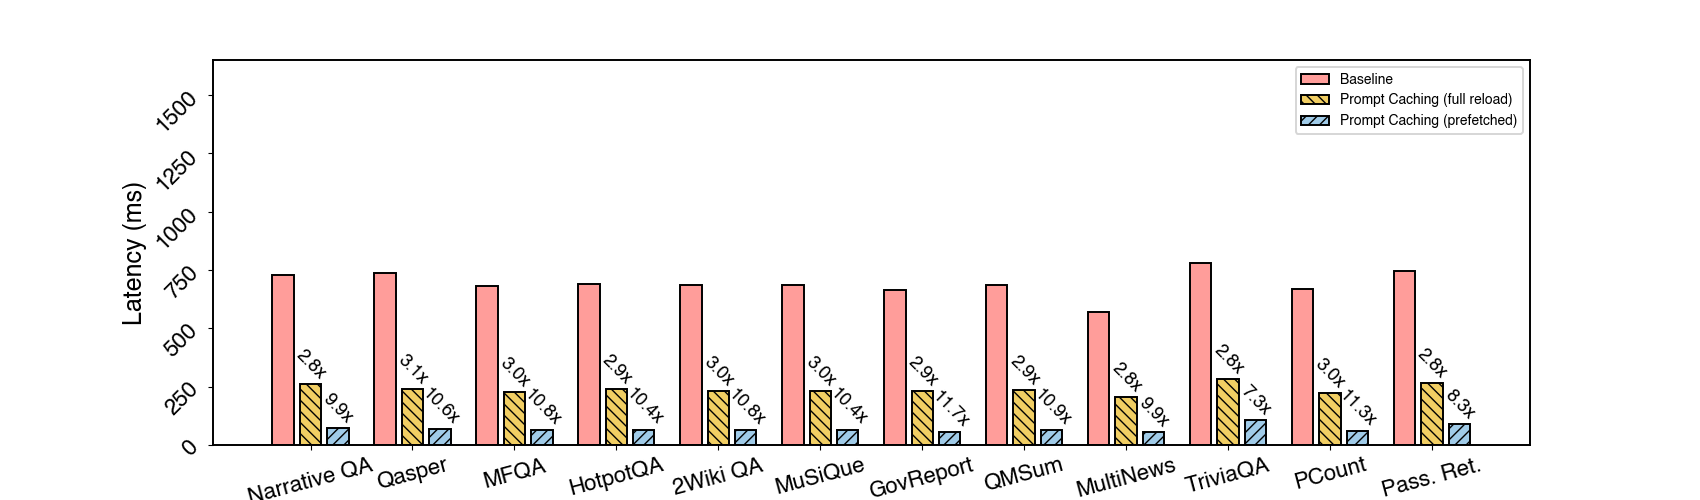}
\caption{Latency benchmark results on Nvidia RTX 4090 GPU.}
\label{fig:appendix-gpu-latency-rtx4090}
\end{figure*}

\begin{figure*}[]
\centering
\vspace{-10pt}
\includegraphics[width=0.95\textwidth]{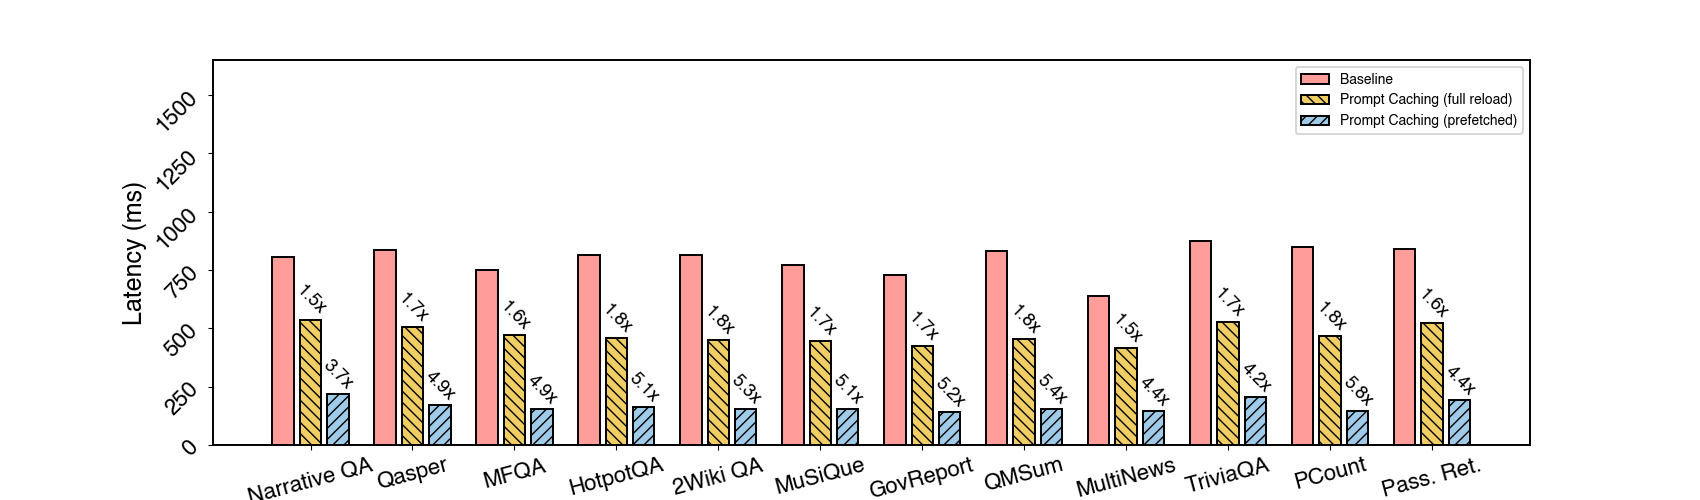}
\caption{Latency benchmark results on Nvidia A100 GPU.}
\label{fig:appendix-gpu-latency-a100}
\end{figure*}

\begin{figure*}[]
\centering

\includegraphics[width=0.95\textwidth]{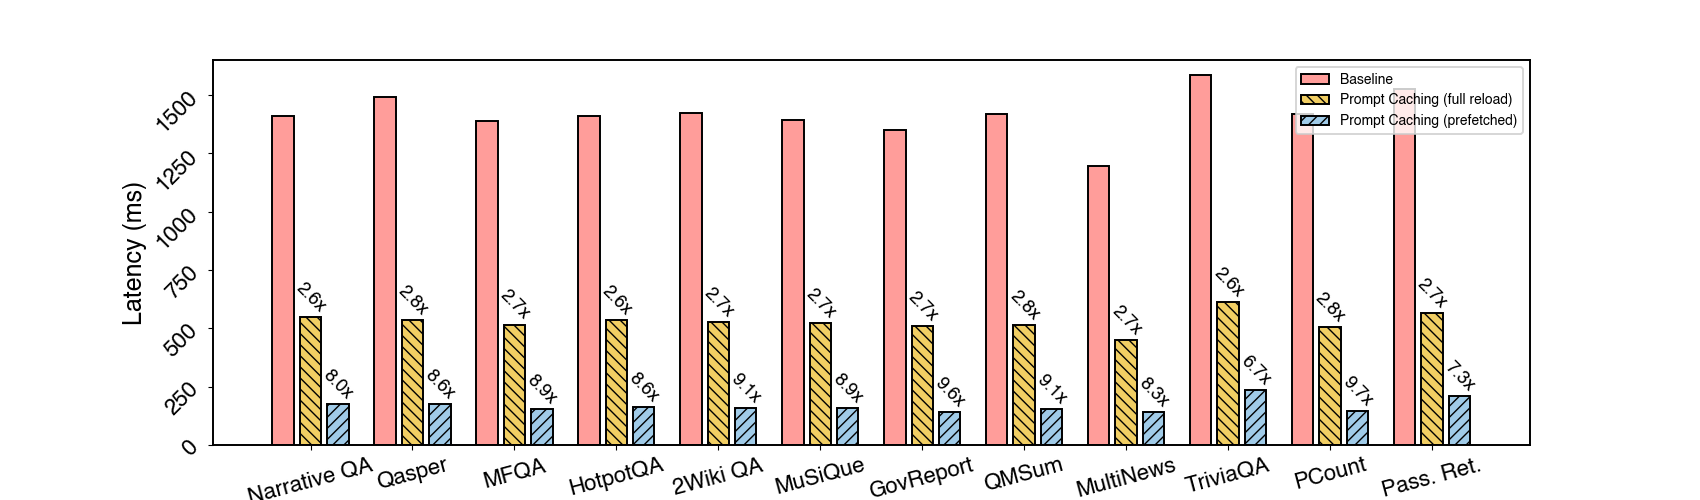}
\vspace{-10pt}
\caption{Latency benchmark results on Nvidia A40 GPU.}
\label{fig:appendix-gpu-latency-a40}
\end{figure*}

\begin{figure*}[]
\centering
\vspace{-10pt}
\includegraphics[width=0.95\textwidth]{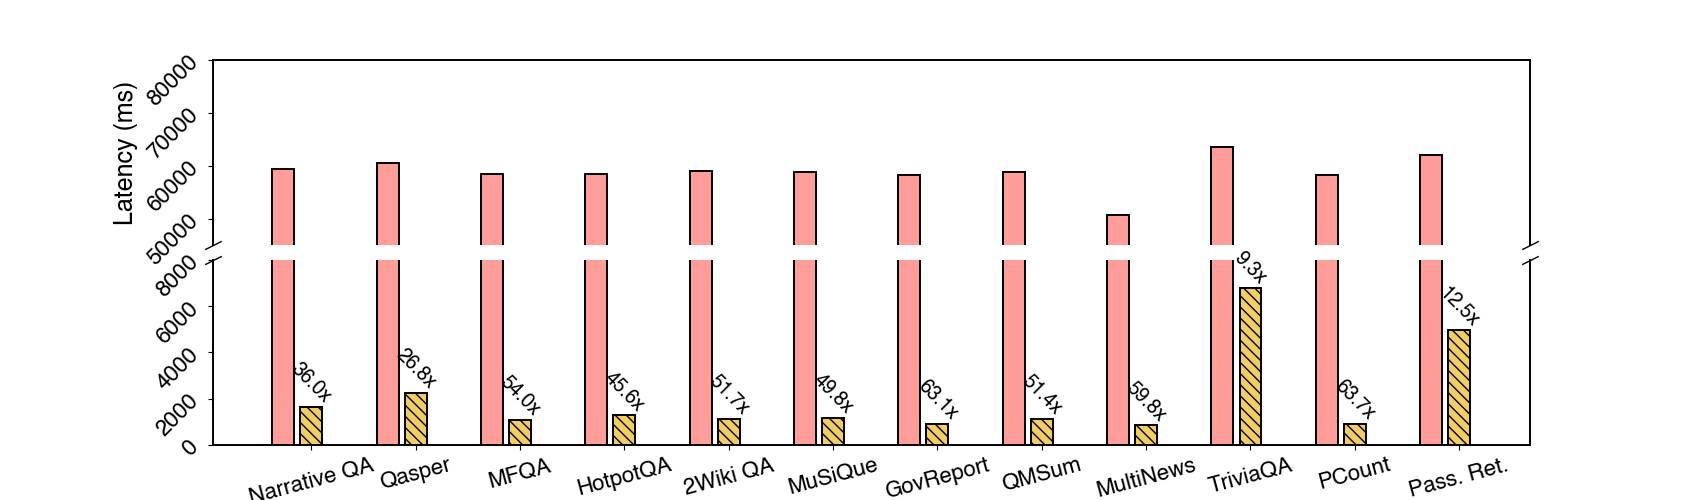}
\caption{Latency benchmark results on Intel i9-13900K CPU with 5600MT/s DDR5 RAM.}
\label{fig:appendix-cpu-latency-intel}
\end{figure*}

\begin{figure*}[]
\centering
\vspace{-10pt}
\includegraphics[width=0.95\textwidth]{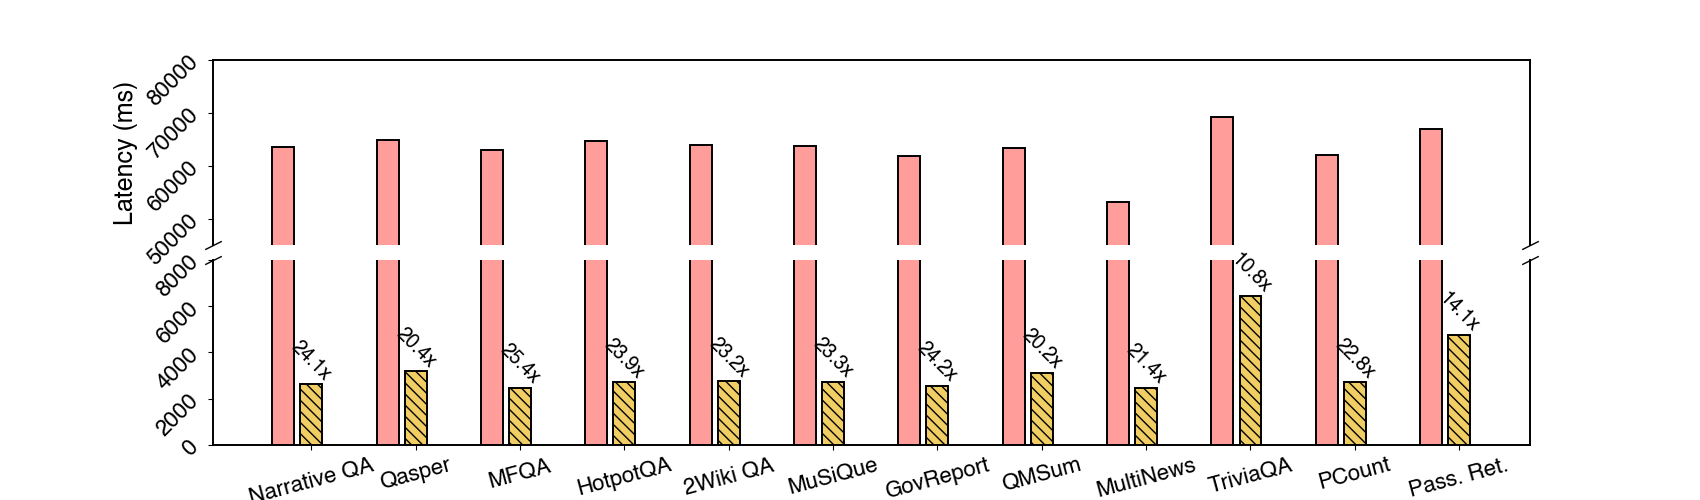}
\caption{Latency benchmark results on AMD Ryzen 9 7950X CPU with 3600 MT/s DDR4 RAM.}
\label{fig:appendix-cpu-latency-amd}
\end{figure*}

\begin{table*}[!b]
\vspace{-30pt}
\centering
\small
\begin{tabular}{@{}c|c|ll|ll|ll|ll@{}}
\toprule
Dataset           & Metric  & \multicolumn{2}{c|}{Llama2 7B} & \multicolumn{2}{c|}{Llama2 13B} & \multicolumn{2}{c|}{MPT 7B} & \multicolumn{2}{c}{Falcon 7B} \\ \midrule
                  &         & Baseline       & Cached       & Baseline        & Cached       & Baseline      & Cached     & Baseline       & Cached       \\ \midrule
Narrative QA       & F1      & 19.93          & 19.38        & 20.37           & 19.94        & 10.43         & 11.33      & 7.14           & 8.87         \\
Qasper            & F1      & 17.98          & 19.31        & \textbf{20.90}           & 17.79        & 10.08         & \textbf{13.71}      & 10.64          & 8.90         \\
Multi-field QA (MFQA)     & F1      & 28.61          & 29.64        & 32.12           & 32.37        & 25.15         & 27.45      & 17.49          & 16.65        \\
HotpotQA          & F1      & 18.32          & 19.34        & 22.21           & 23.35        & 18.97         & 20.11      & 12.37          & 13.22        \\
2 Wiki Multi-Hop QA   & F1      & \textbf{16.63}          & 13.95        & 14.59           & \textbf{17.69}        & 10.44         & \textbf{13.70}      & 14.42          & 15.07        \\
MuSiQue           & F1      & 7.31           & 8.57         & 10.03           & 12.14        & 7.38          & 7.32       & 4.81           & 5.86         \\
GovReport         & Rouge L & 24.67          & 25.37        & 28.13           & 28.18        & 26.96         & 27.49      & 22.39          & 23.40        \\
QMSum             & Rouge L & 19.24          & 19.46        & 18.80           & 18.82        & 15.19         & 15.51      & 12.84          & 12.96        \\
MultiNews         & Rouge L & 24.33          & 24.22        & 25.43           & 26.23        & 25.42         & 25.66      & 20.91          & 21.19        \\
TriviaQA          & F1      & 13.04          & 12.33        & 23.19           & 22.38        & 10.57         & 9.17       & 13.31          & 11.42        \\
Passage Count (PCount)     & Acc     & 3.33           & 4.00         & 2.26            & 2.95         & 1.53          & 1.81       & 1.55           & 1.59         \\
Passage Retrieval & Acc     & \textbf{7.50}           & 4.25         & \textbf{9.08}            & 6.50         & 3.03          & 3.85       & 3.00           & 3.45         \\
\bottomrule
\end{tabular}
\caption{Accuracy benchmarks on LongBench datasets. We mark the outliers as \textbf{bold}, of which the performance is higher than $2.5$ compared to the counter part.}
\label{table:appendix_accuracy}
\vspace*{28em}
\vfill
\end{table*}
